# Supplementary material for: Analysis of the SBP-SAT Stabilization for Finite Element Methods Part II: Entropy Stability
Source: arXiv:1912.08390 source file (2019-12-18)
Supplement: Supplementary file 1 [file appendix.tex]

\section{Appendix}\label{sec:appendix}

Different from section \ref{sec:non-linear} there are also other possibilities to 
detetermine the boundary operators. However, most of them comes with some restriction 
on the problem or the flux functions. If one consideres for example
a multi-dimensional scalar case, one can use a Taylor series expanons in respect 
to $\bbg(V)\bn:=T_g(V)$ where smoothness is assumed. Another possibility is
if one has some symmetric behaviour of the flux function
and can bring all the information two the boundary. 
This is exactly the key in the investigations of \cite{friedrichs1958symmetric, ern2006discontinuous, nordstrom2017roadmap} 
for the linear case and for the nonlinear case \cite{nordstrom2018energy} where the incompressible Navier-Stokes equation is considered.
However, this is not part of this work. Sometimes it is alos possible to find an recurcsice relation of the flux function
and use this fact in the estimation of the boundary operators. 
